# Supplementary material for: The Chandra Carina Complex Project: Deciphering the Enigma of Carina's Diffuse X-ray Emission
Source: arXiv:1103.0764 ancillary file (2011-03-03)

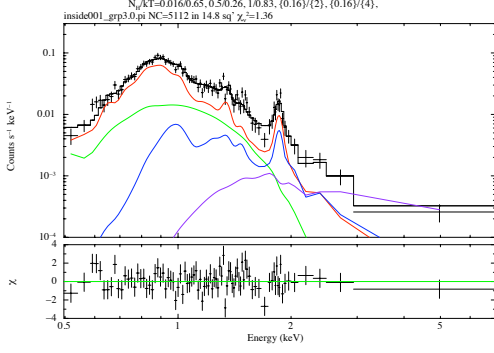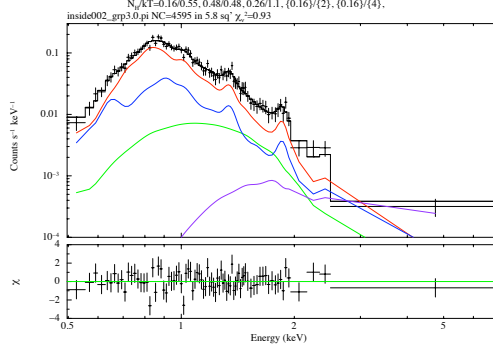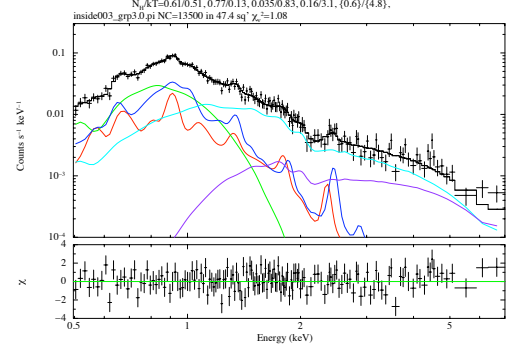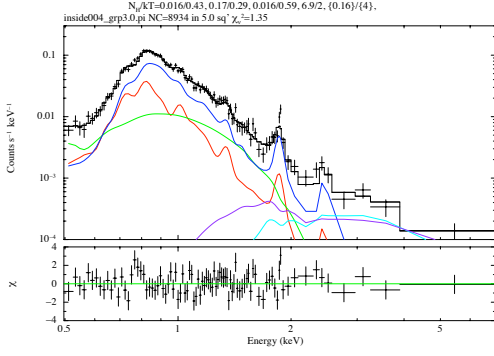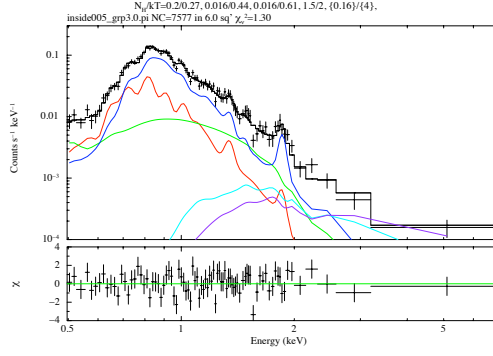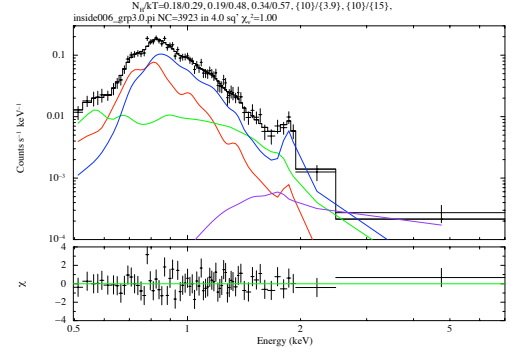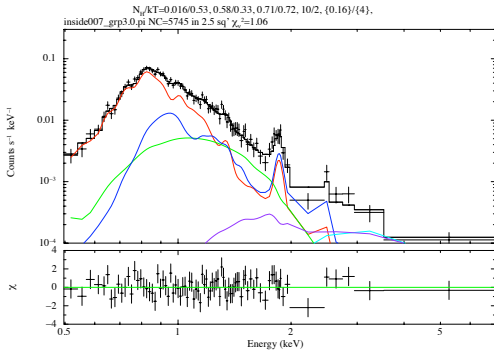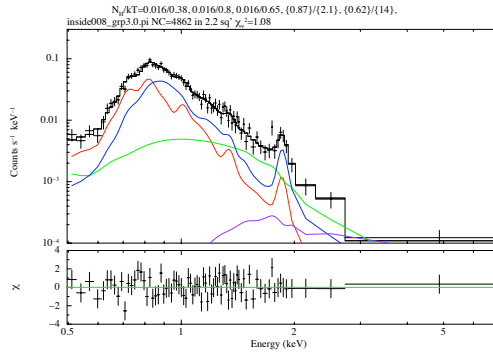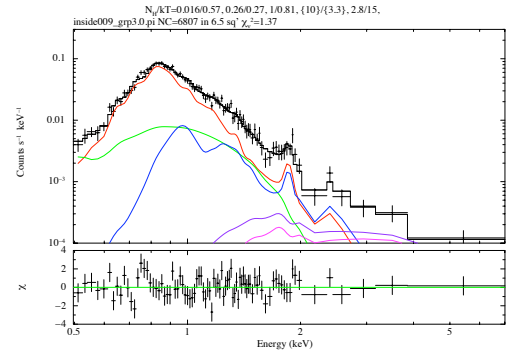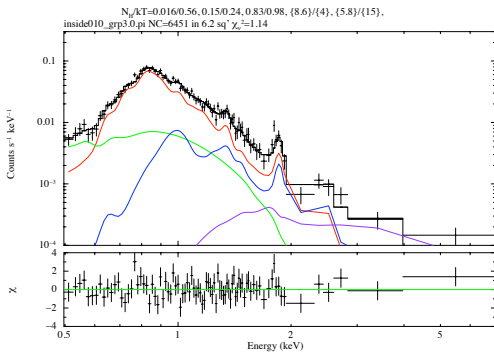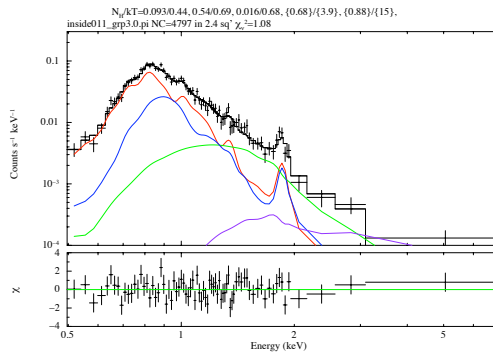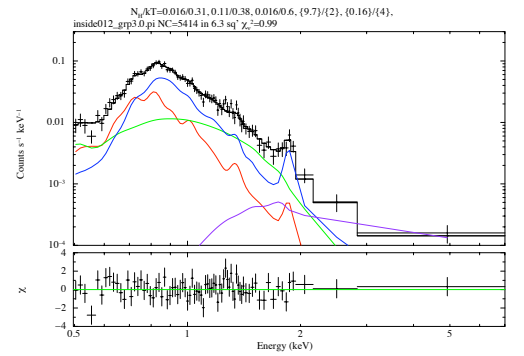

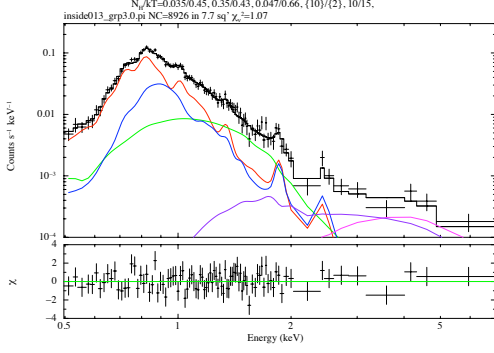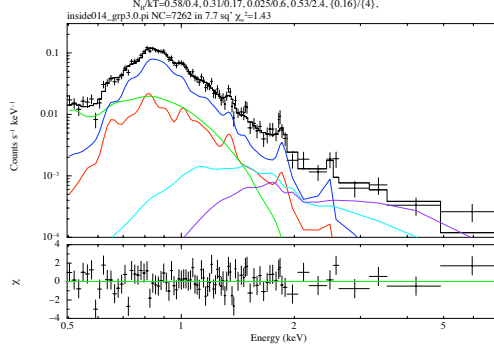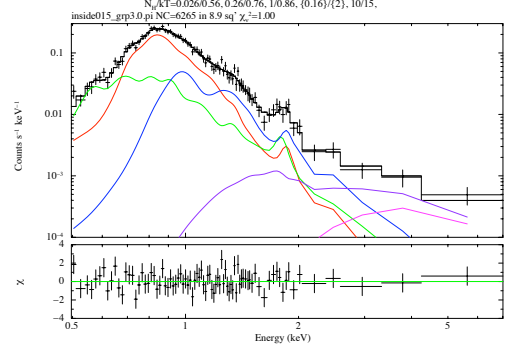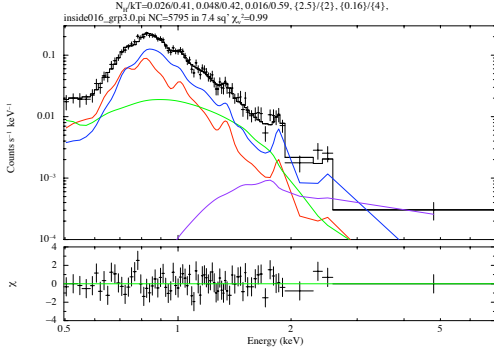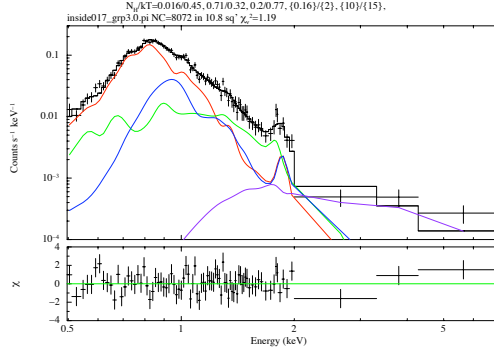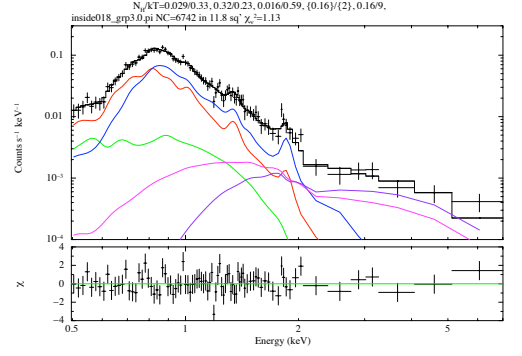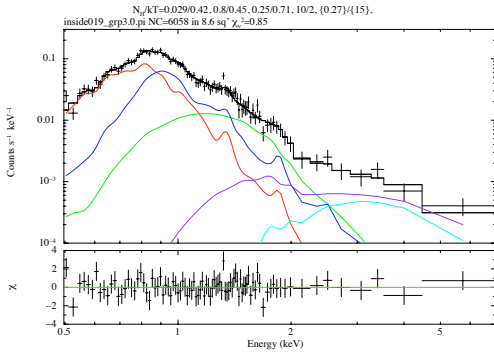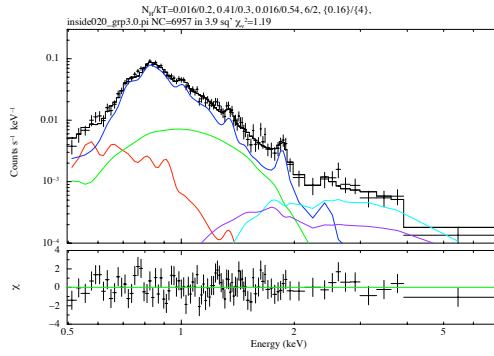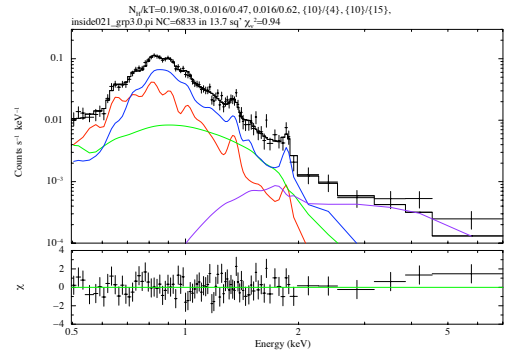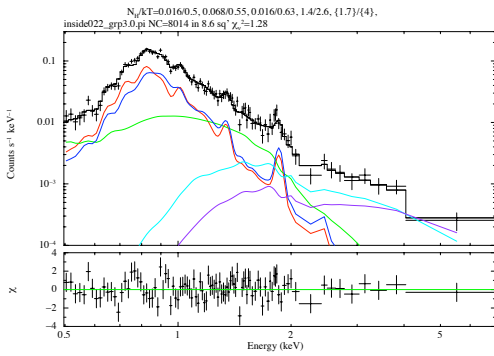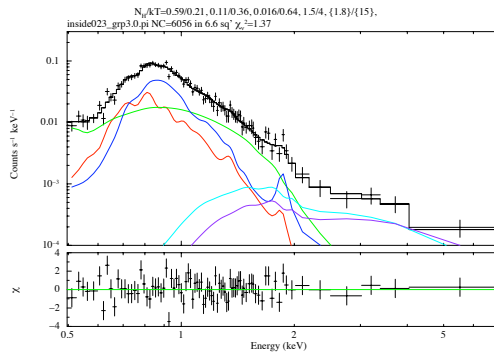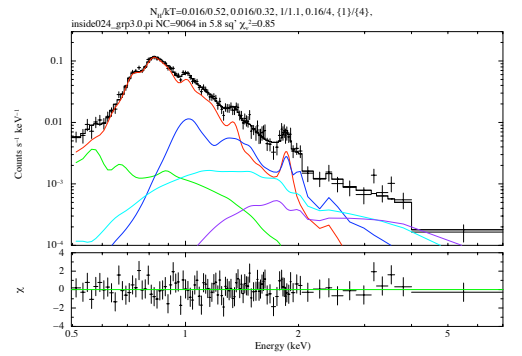

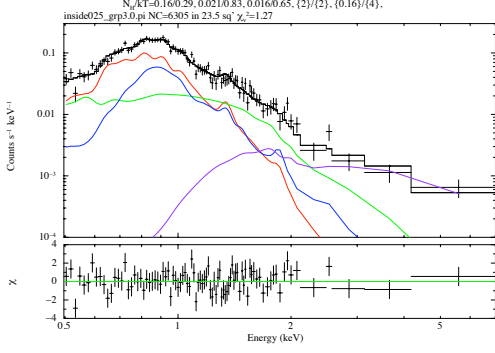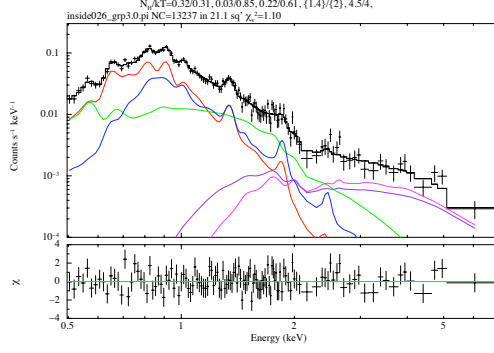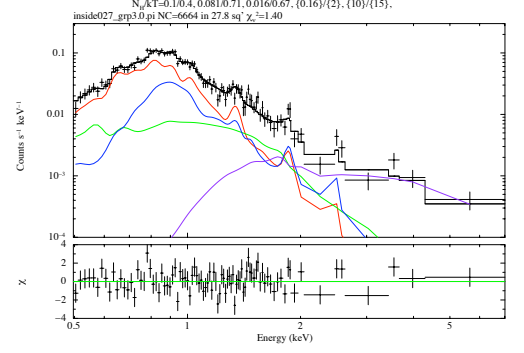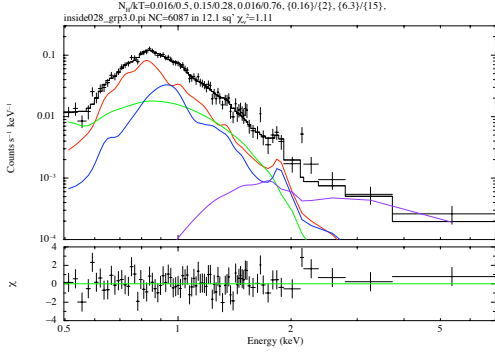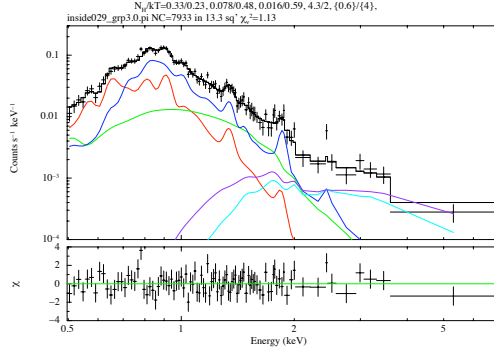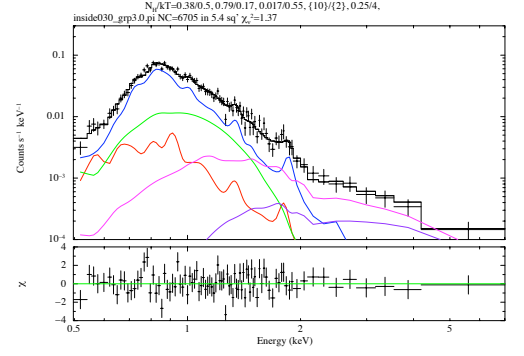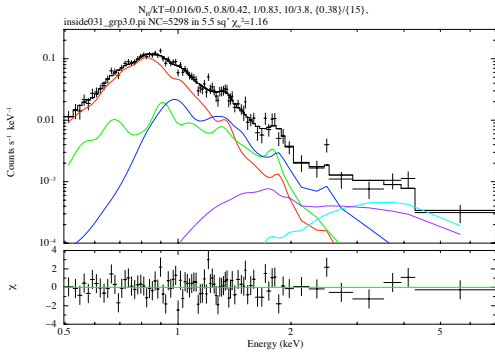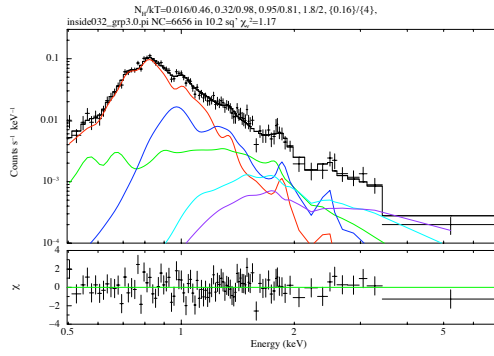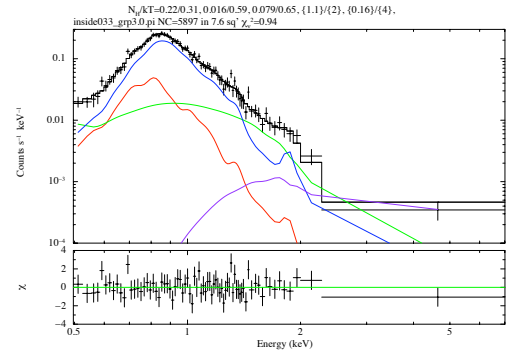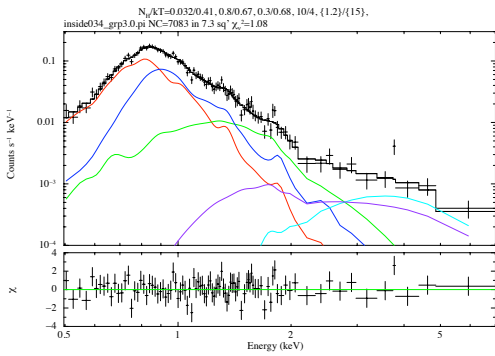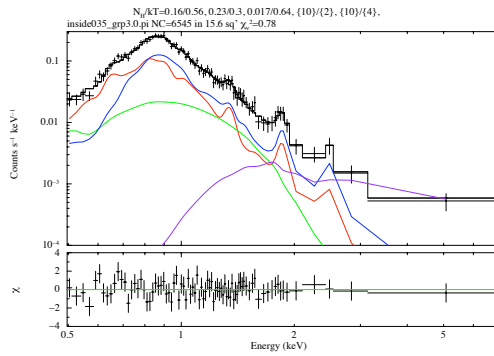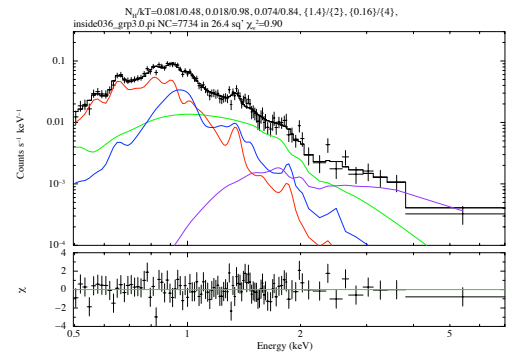

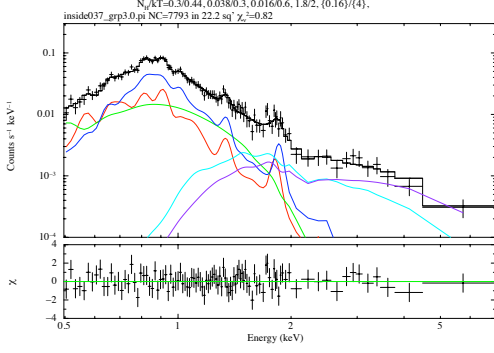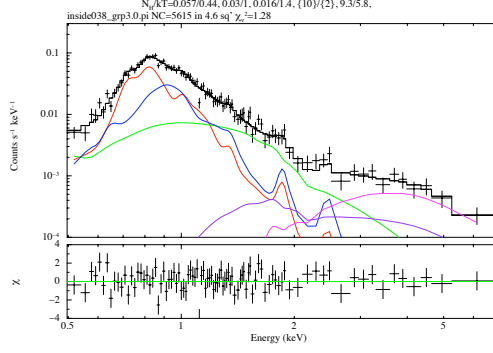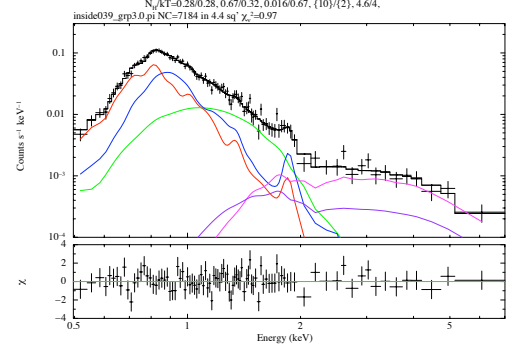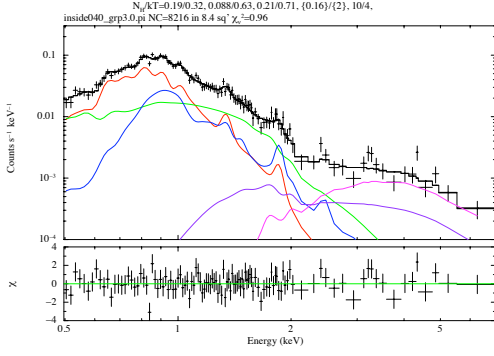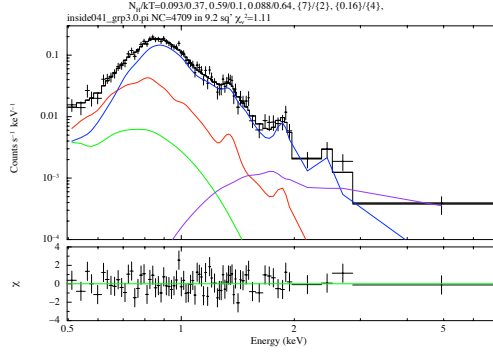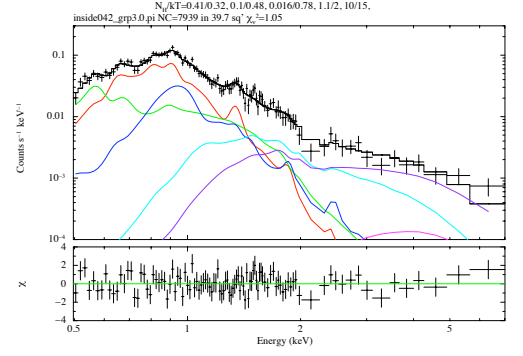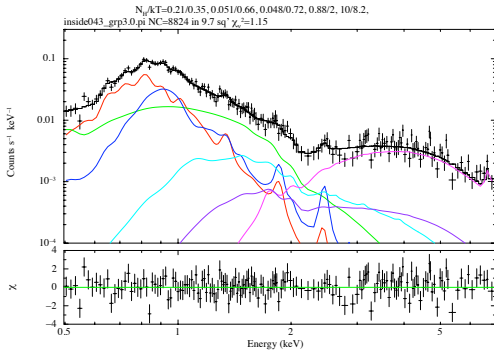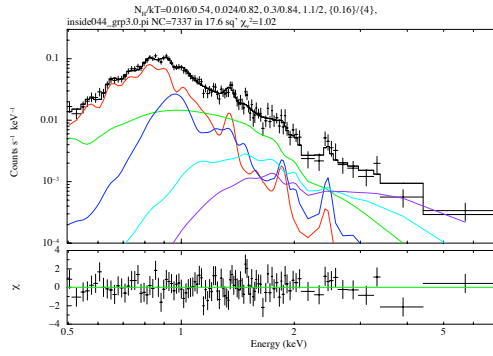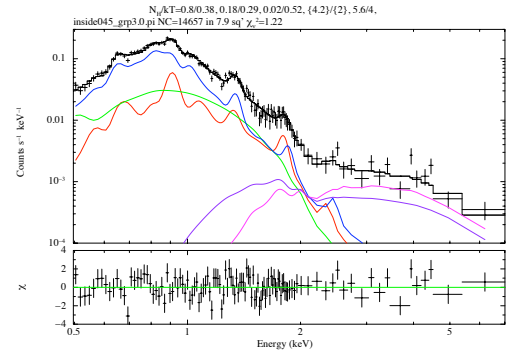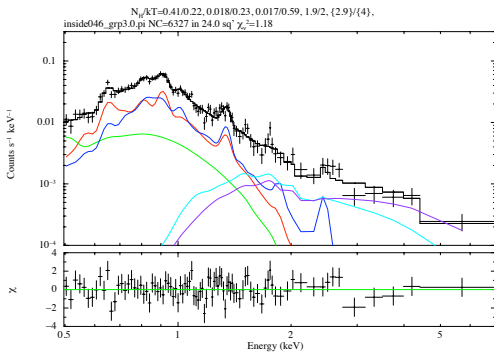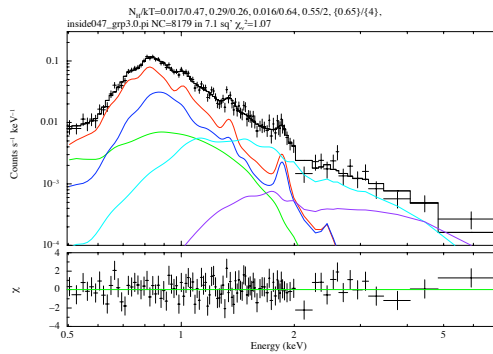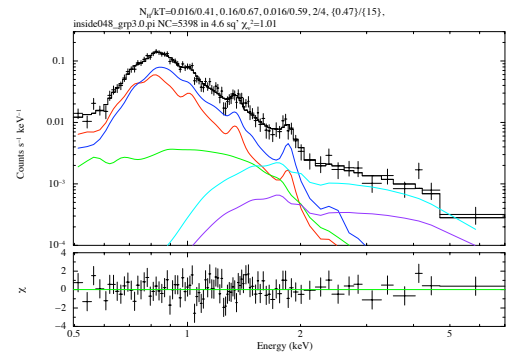

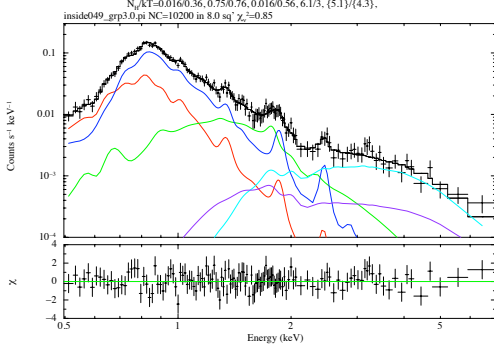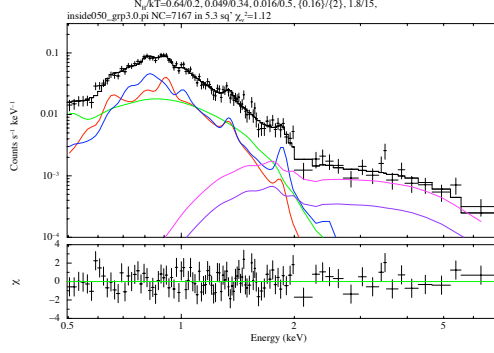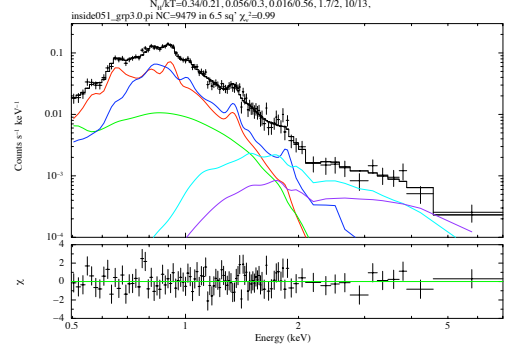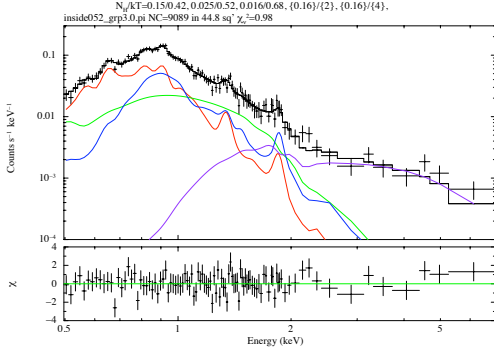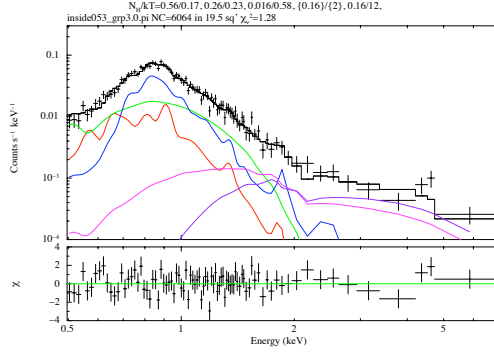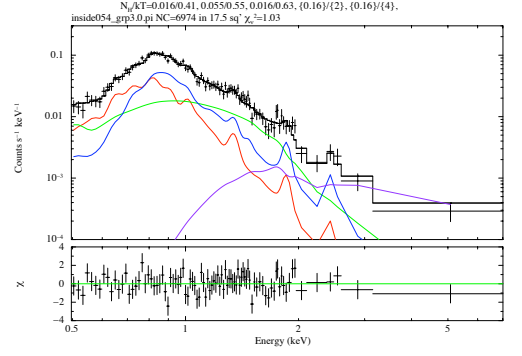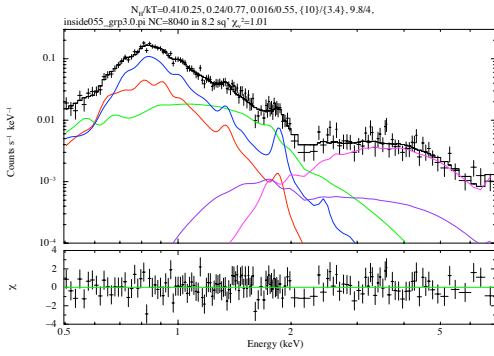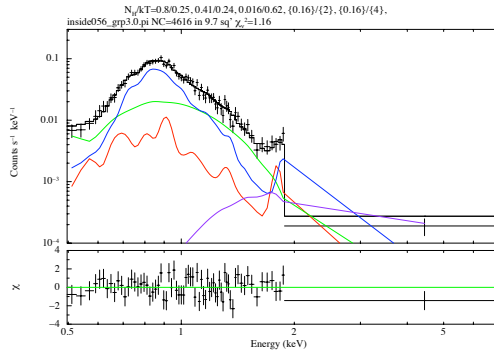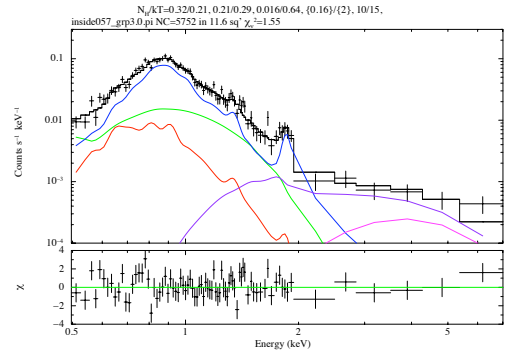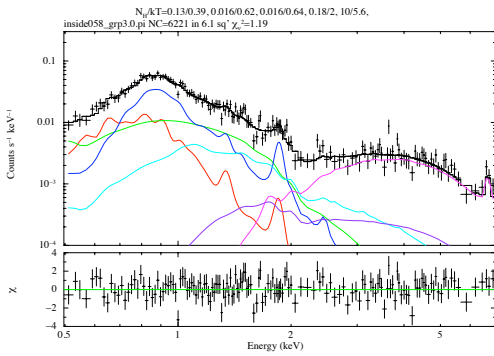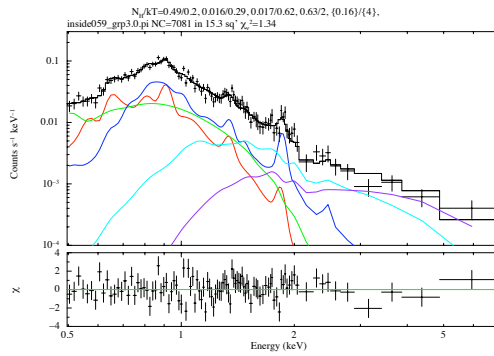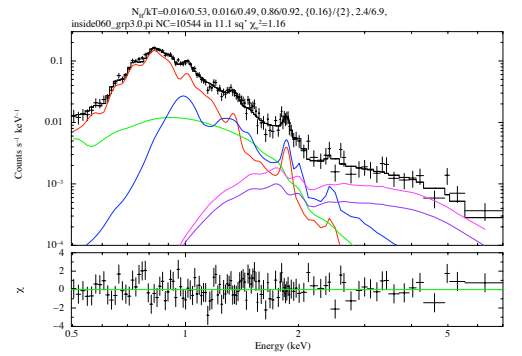

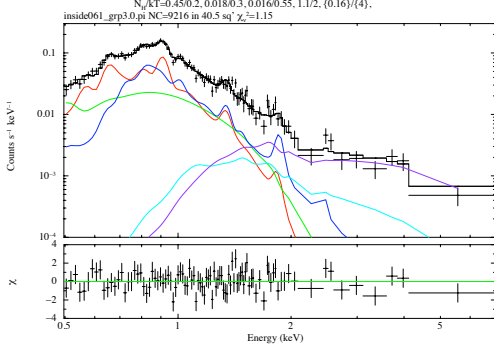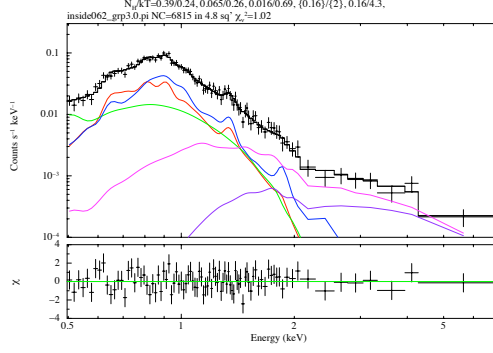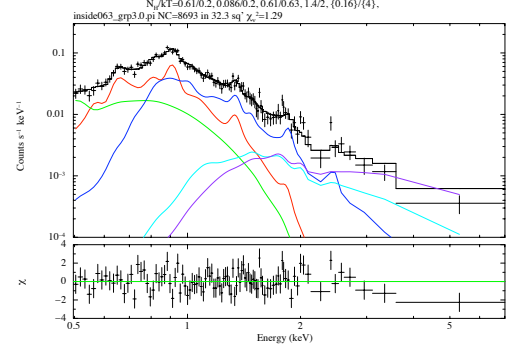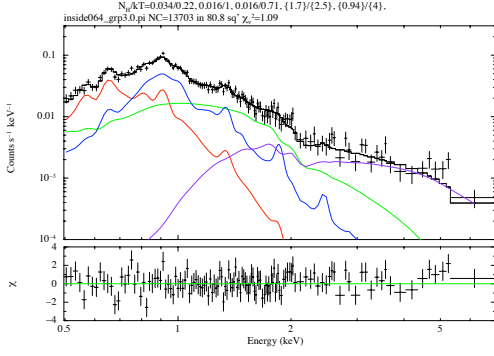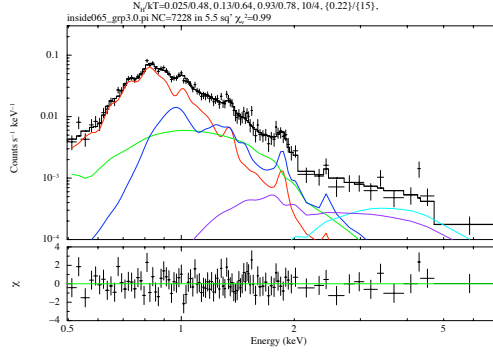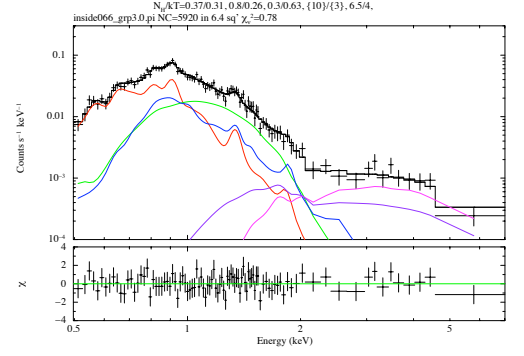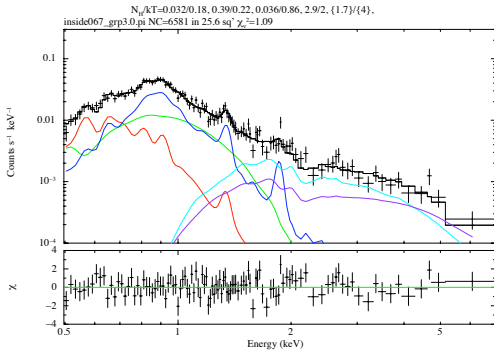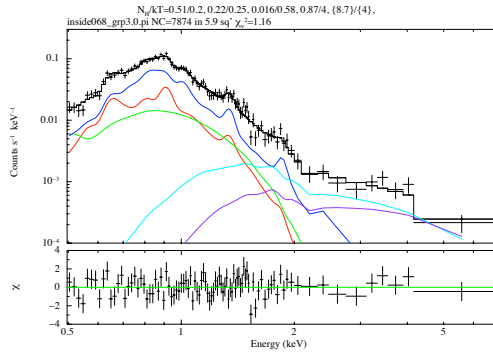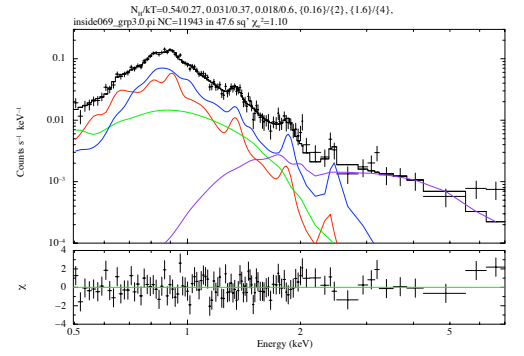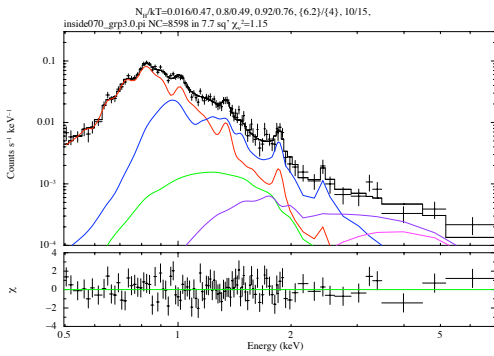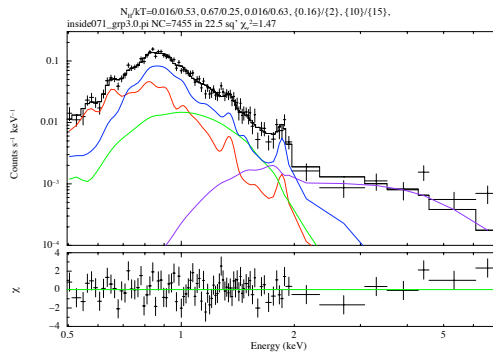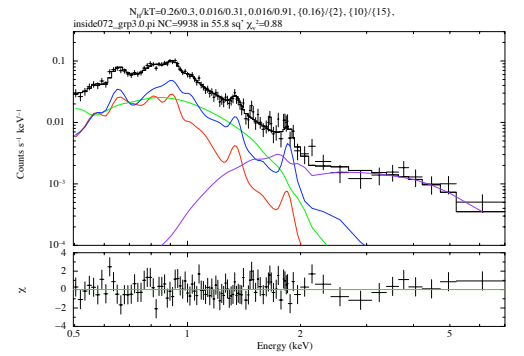

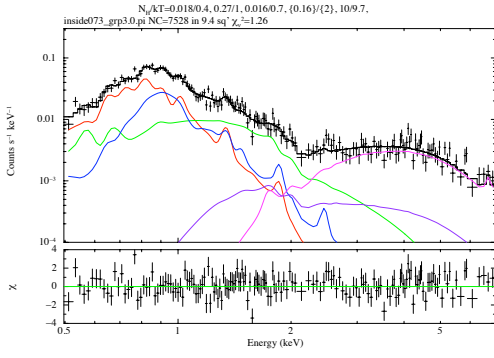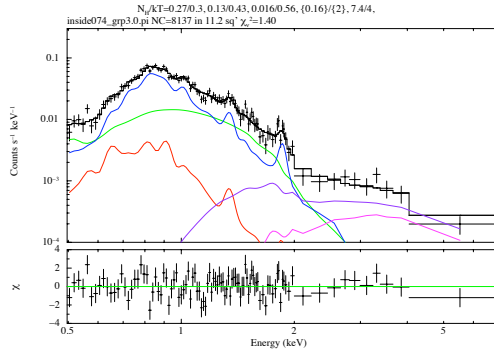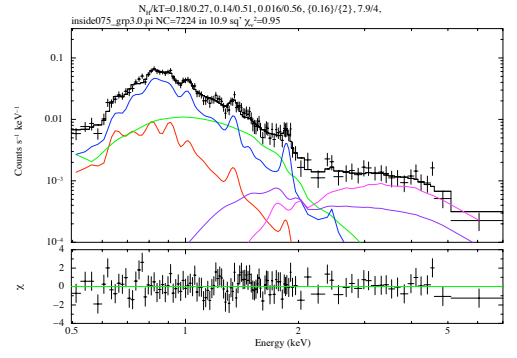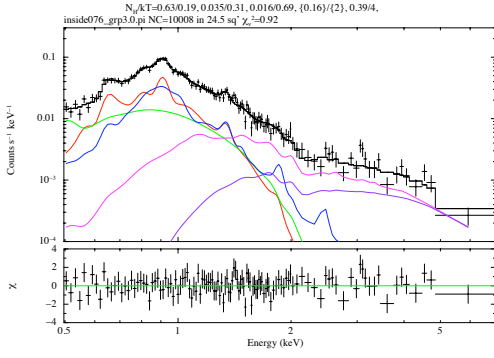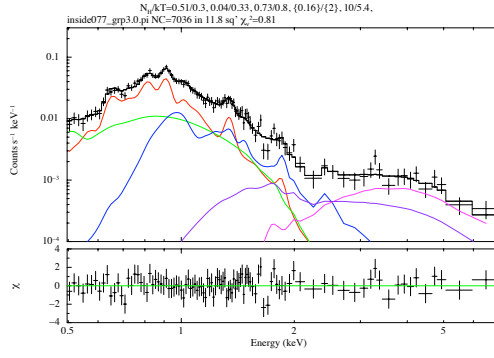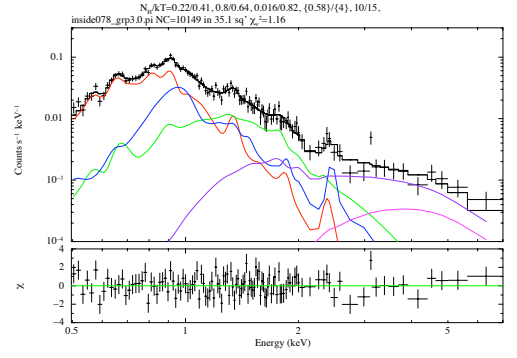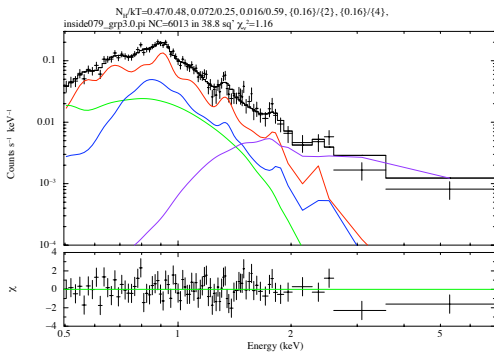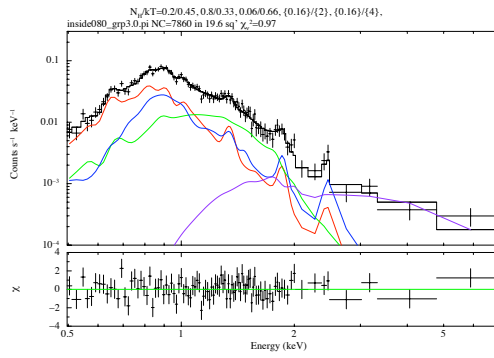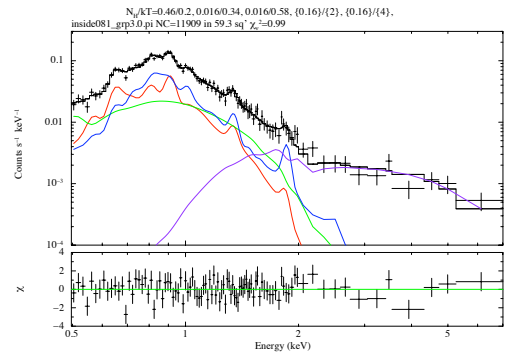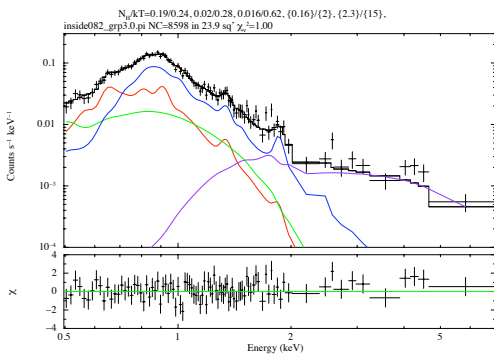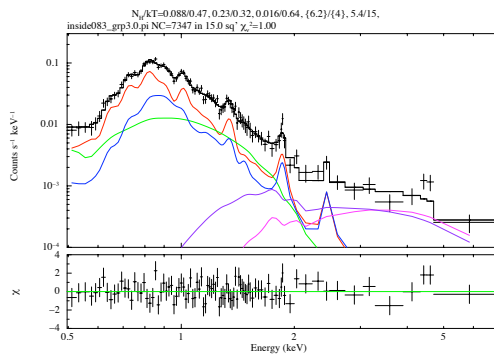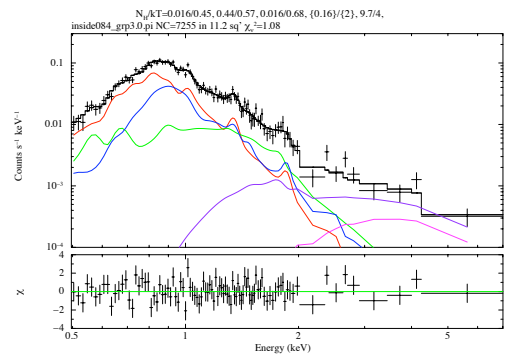



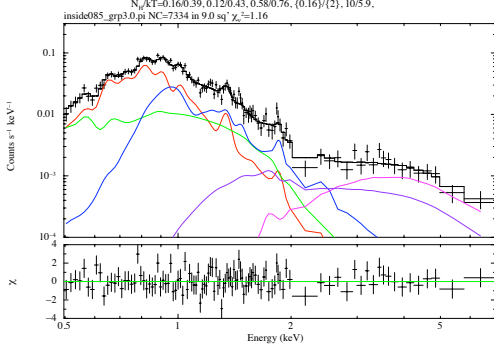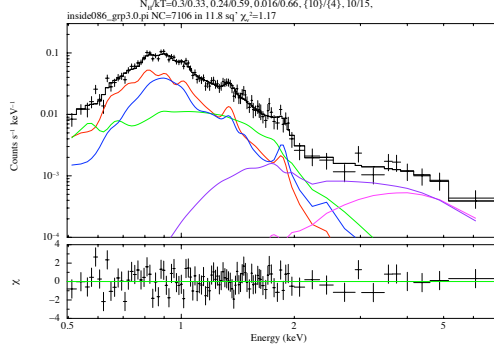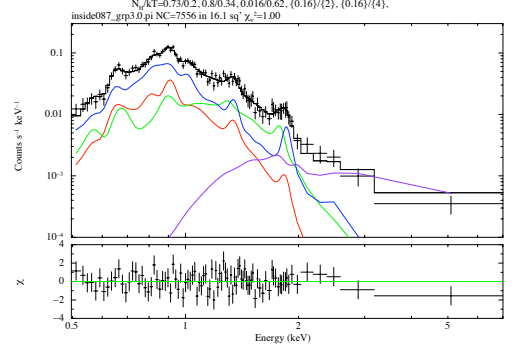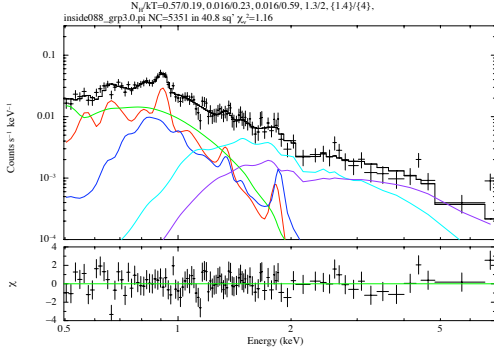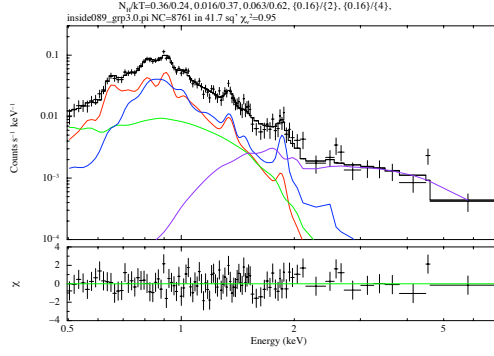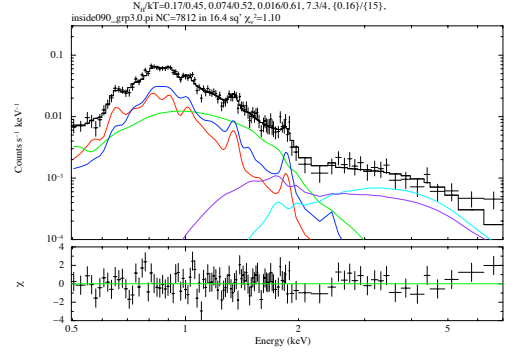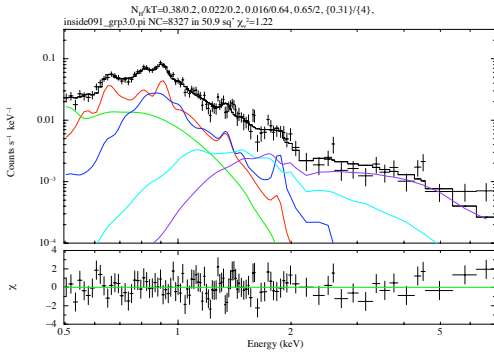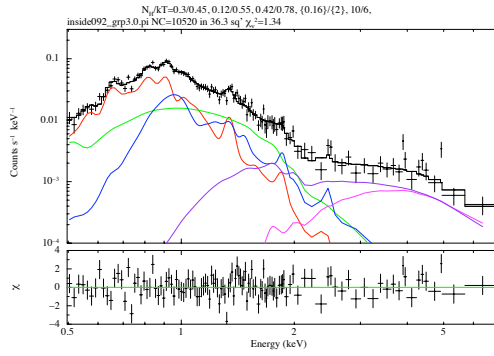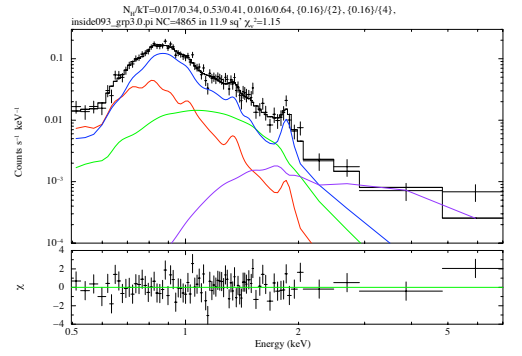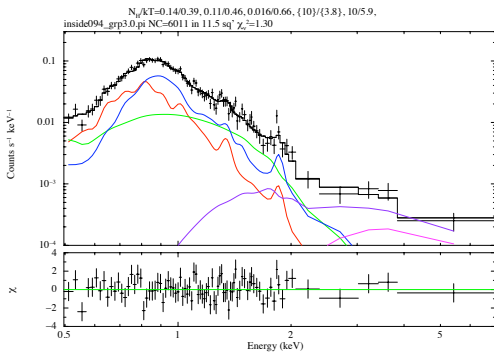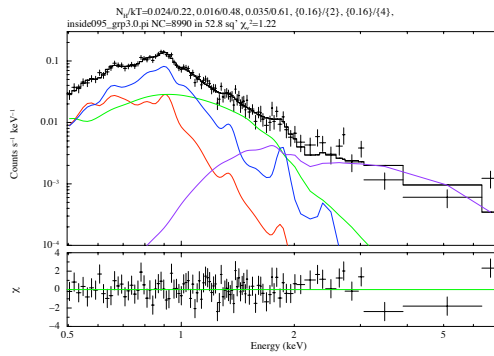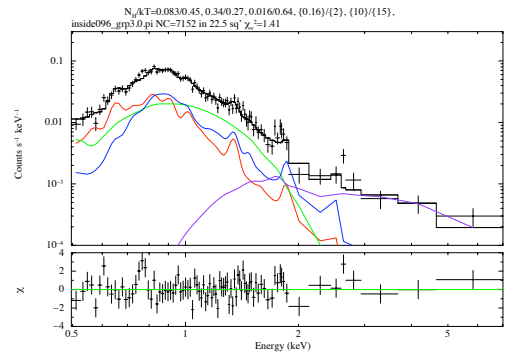



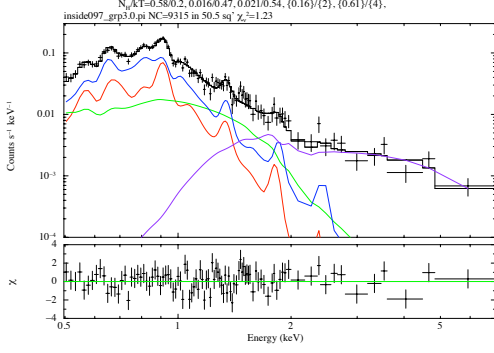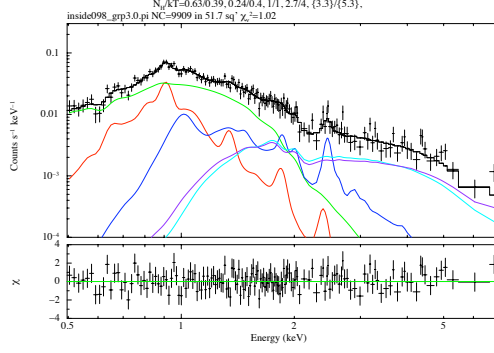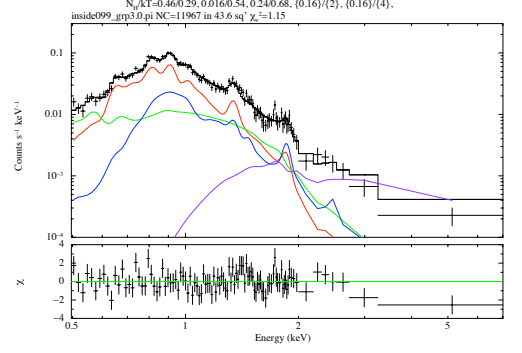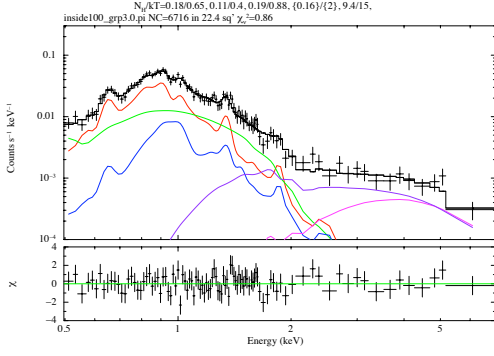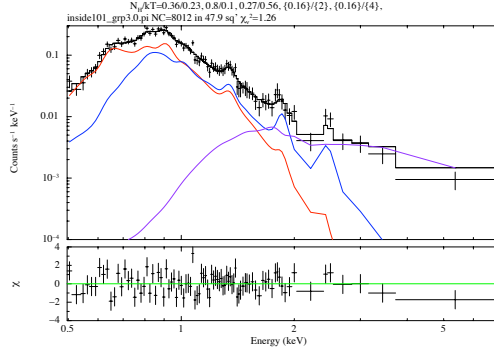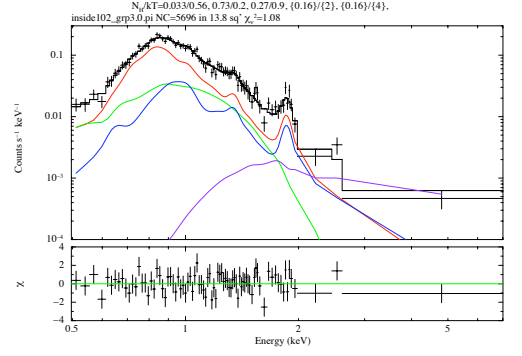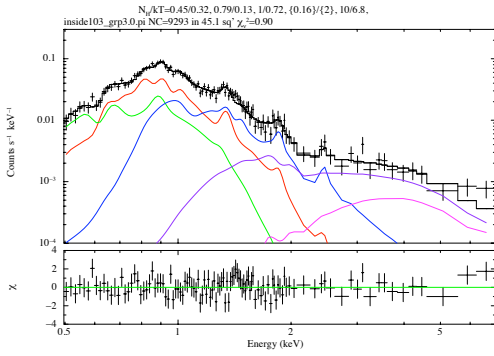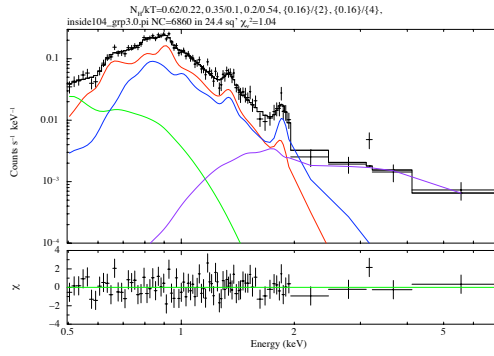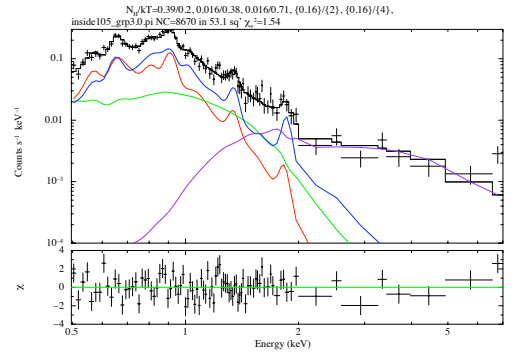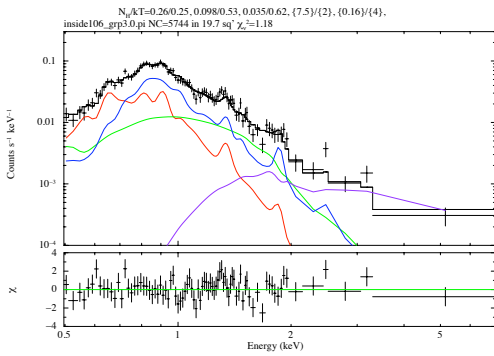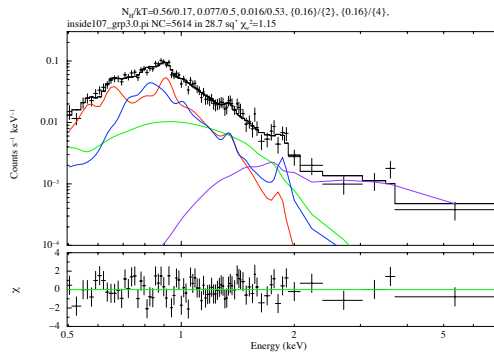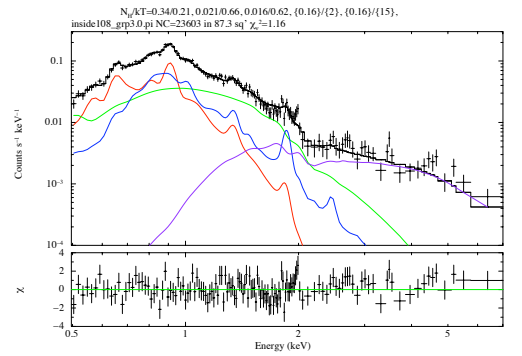

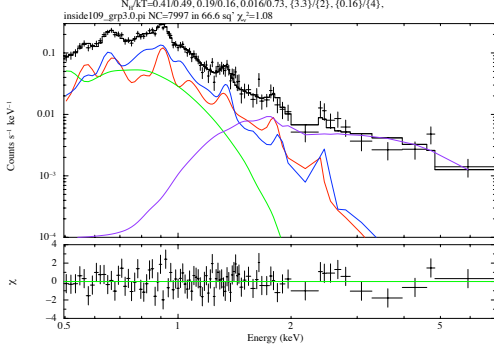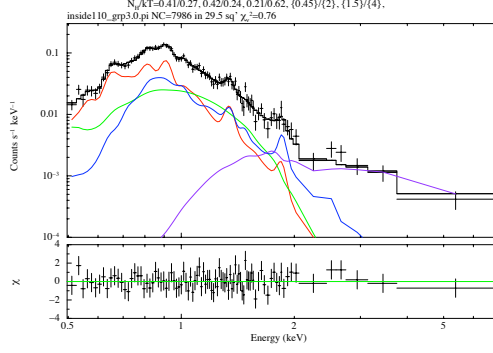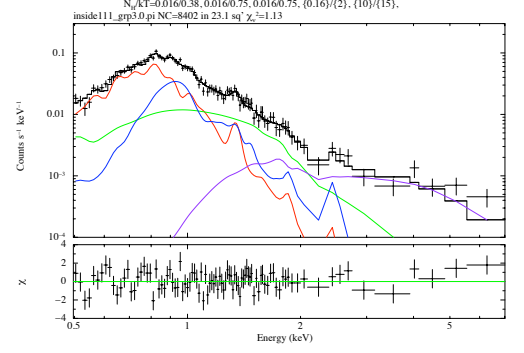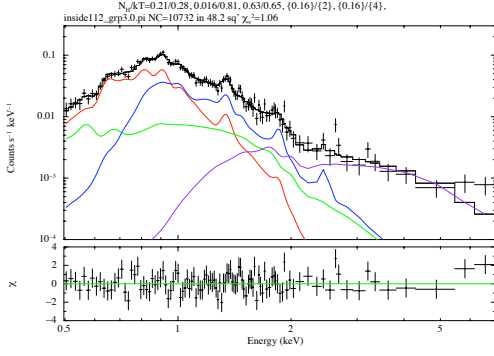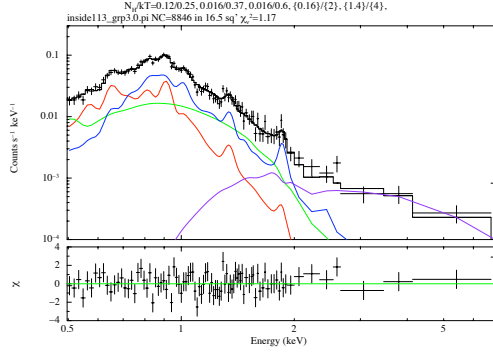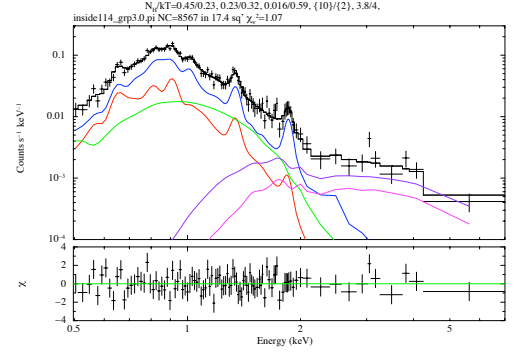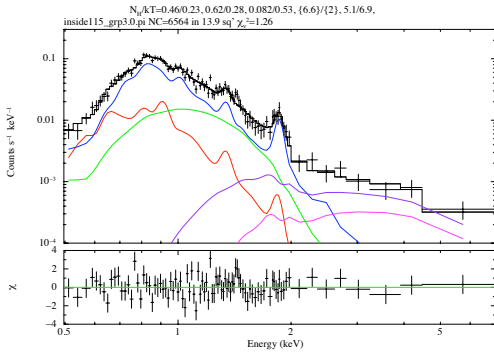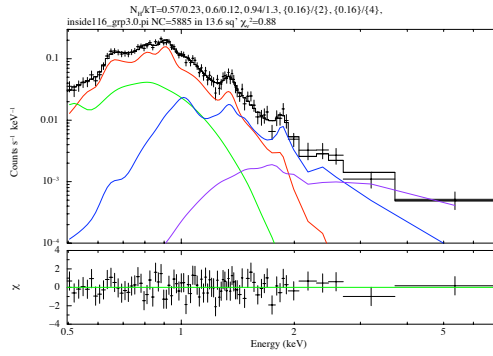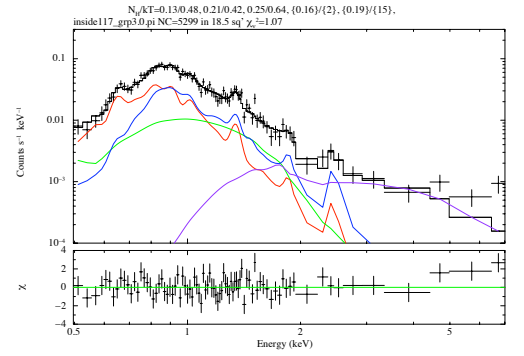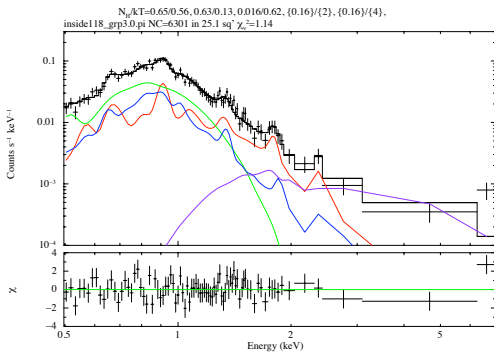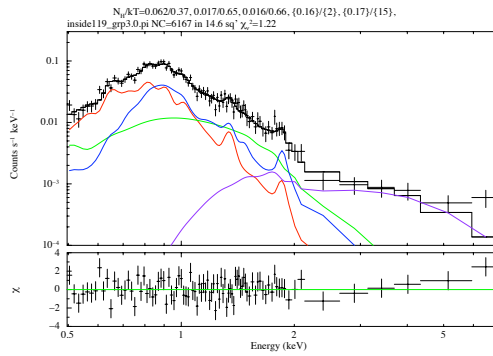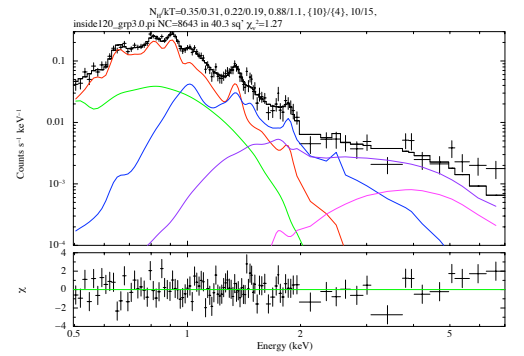

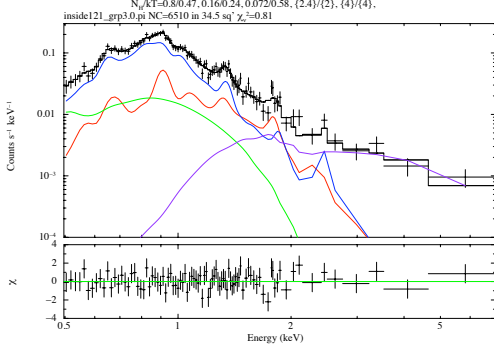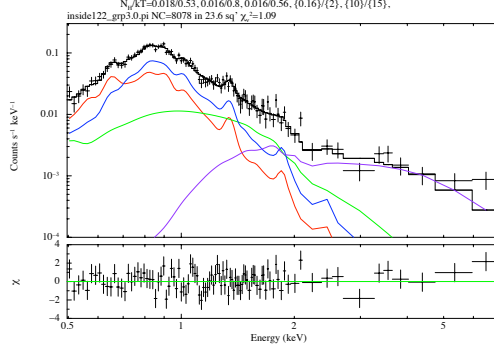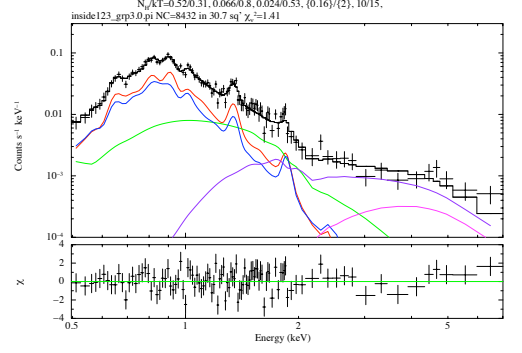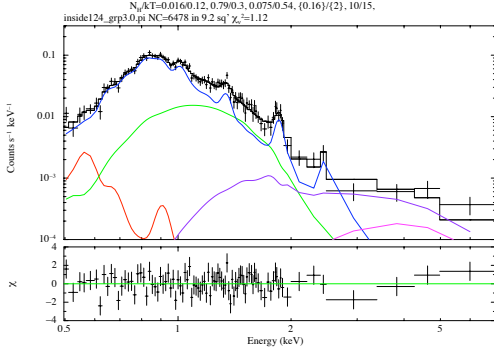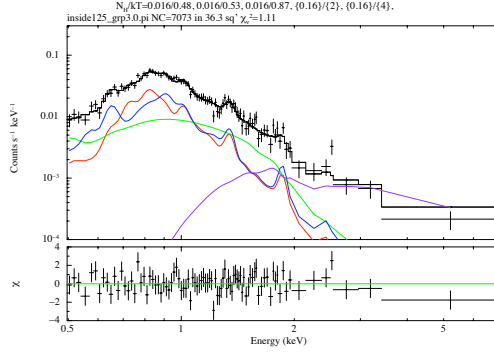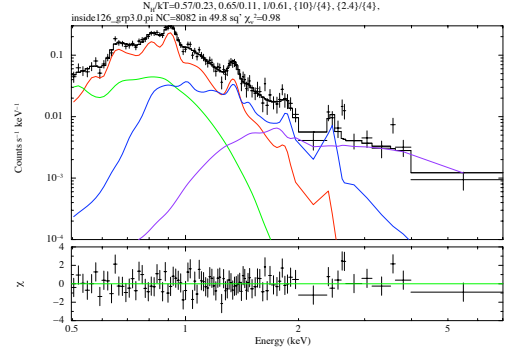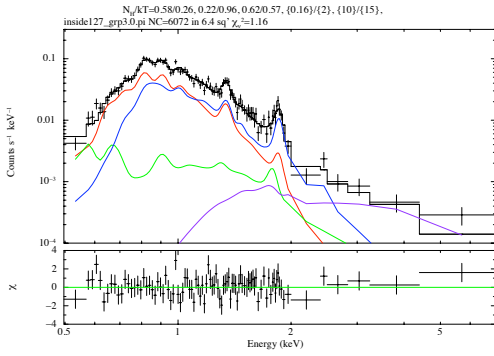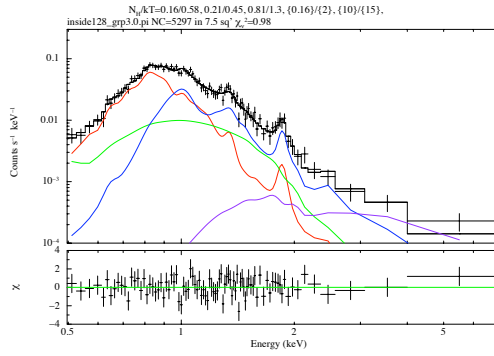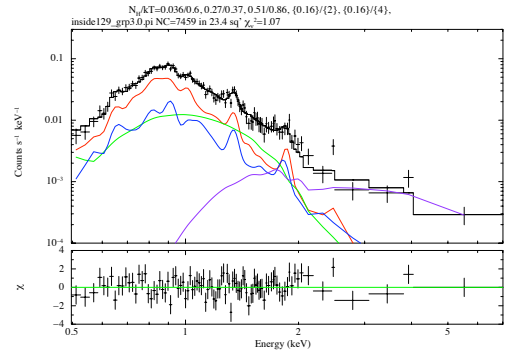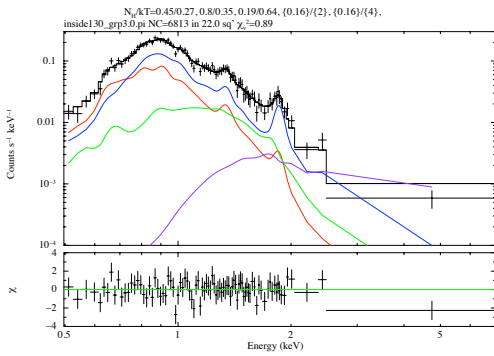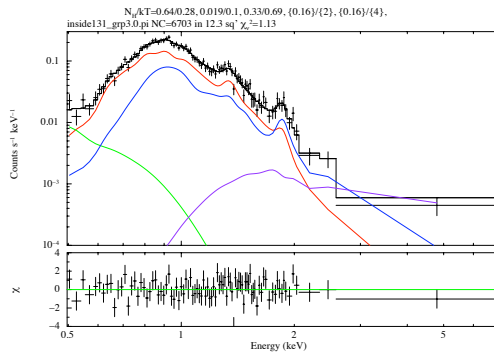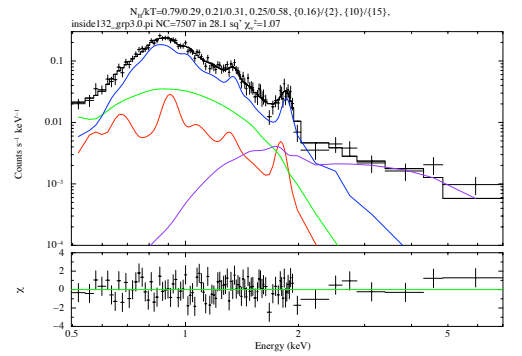

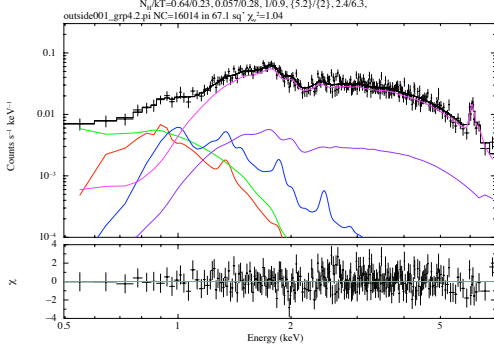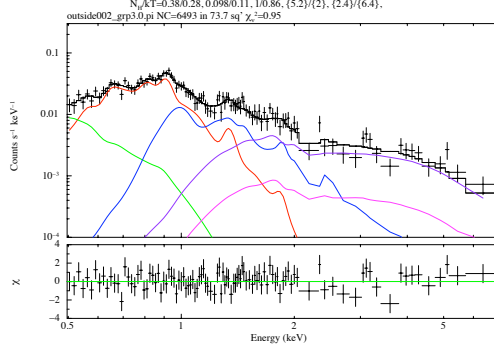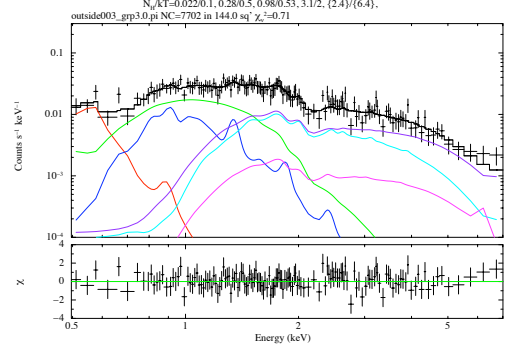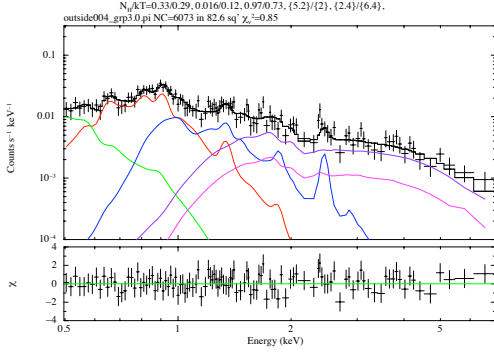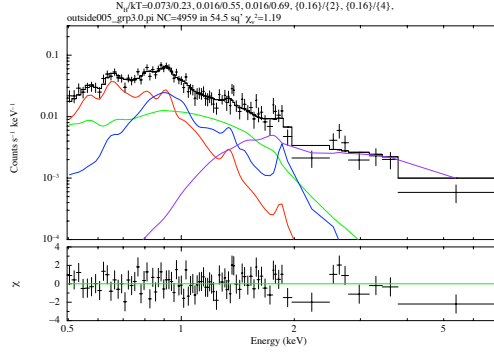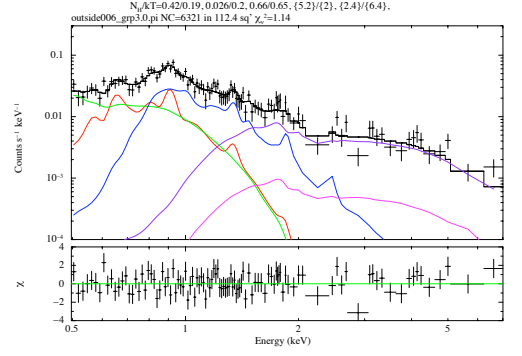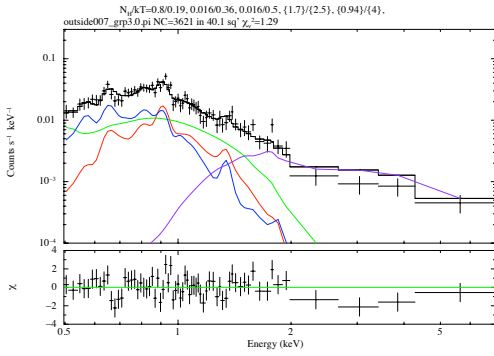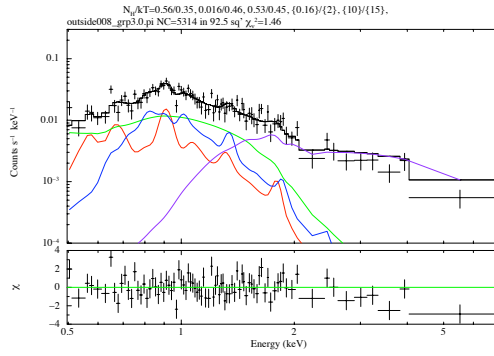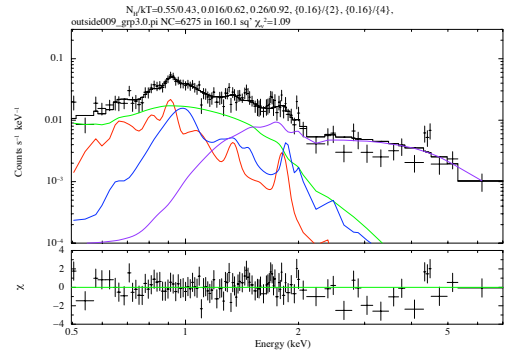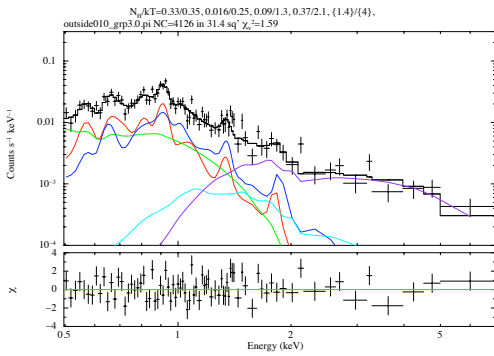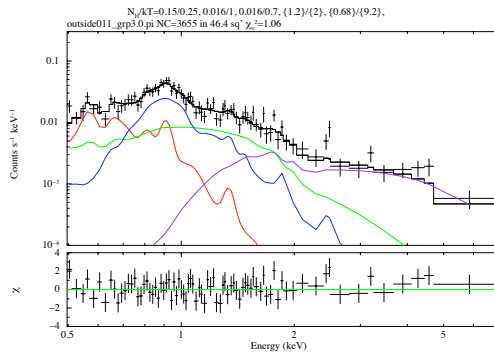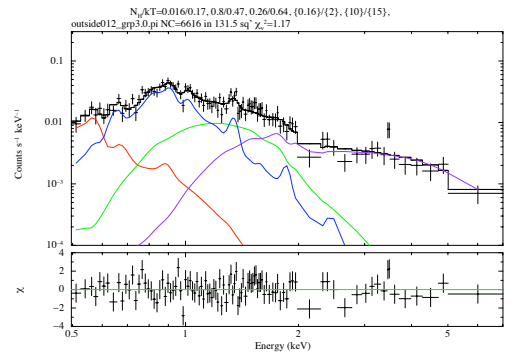

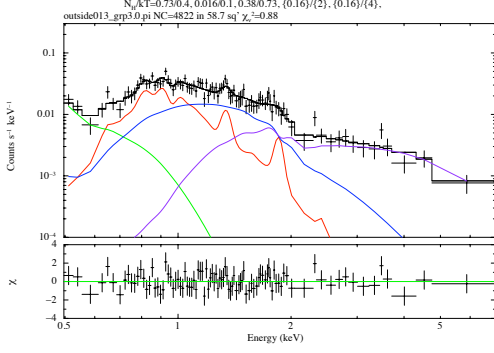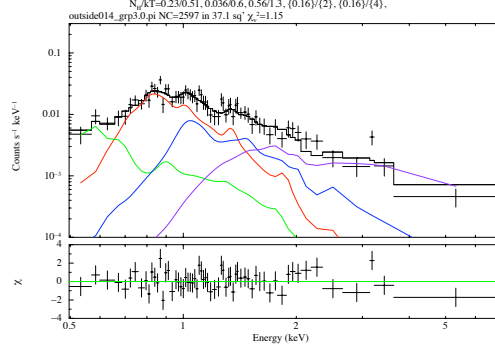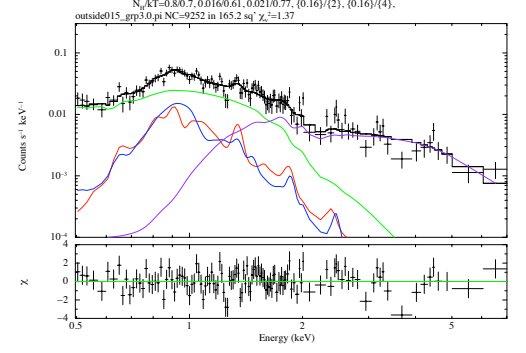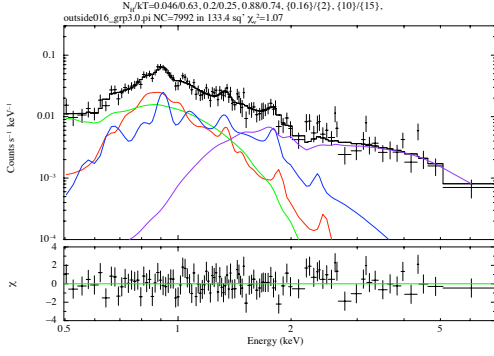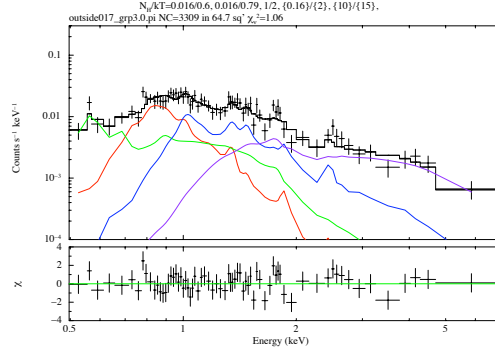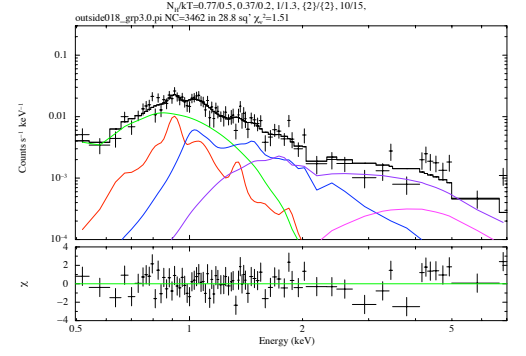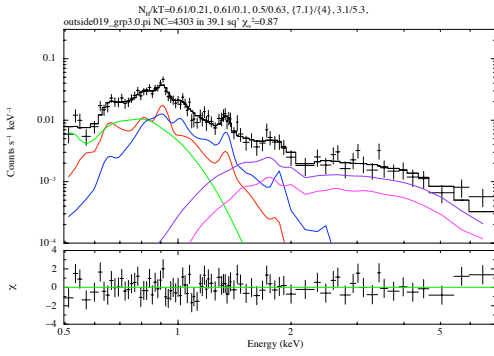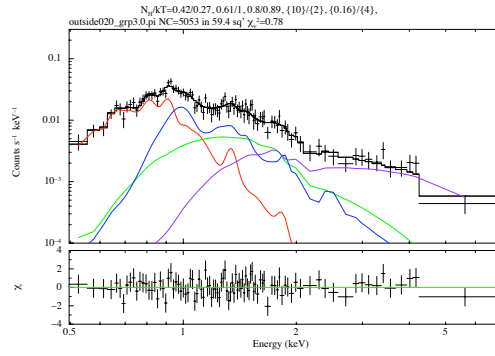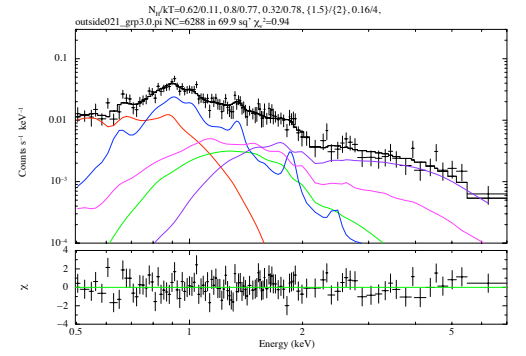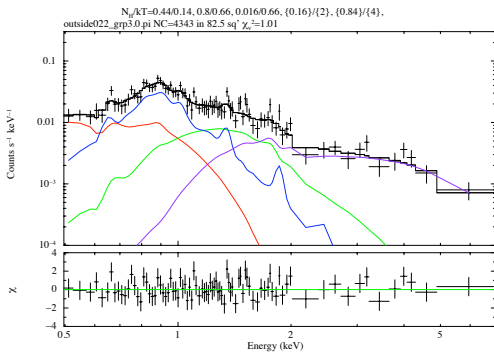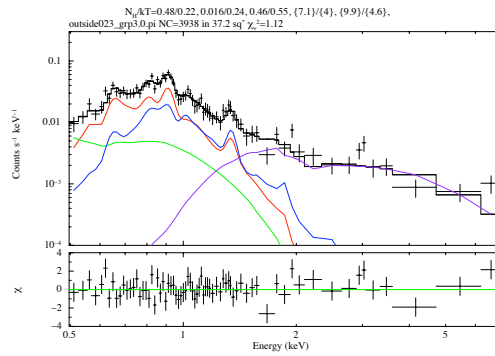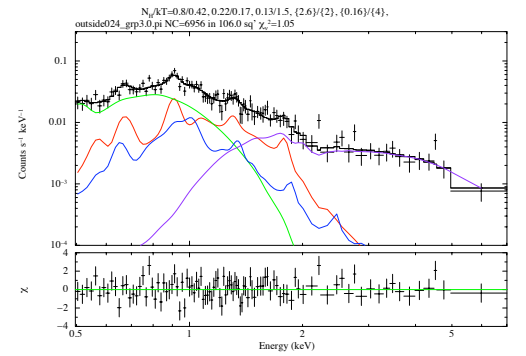

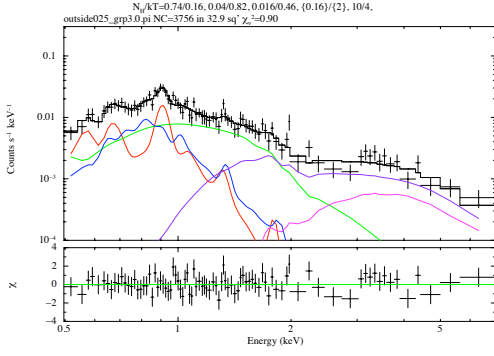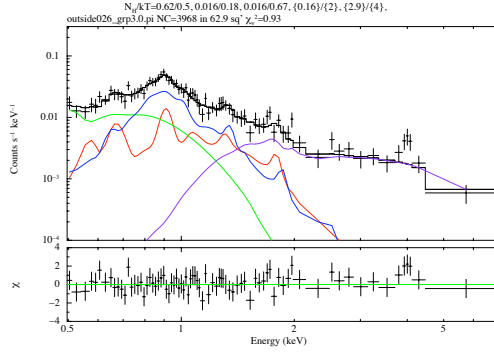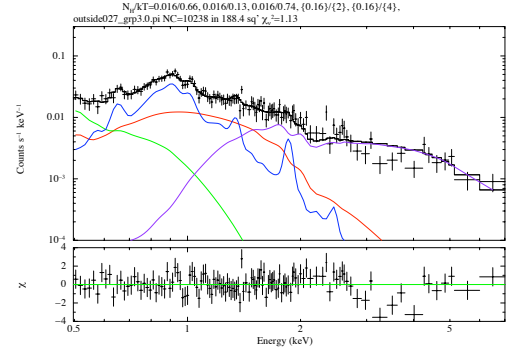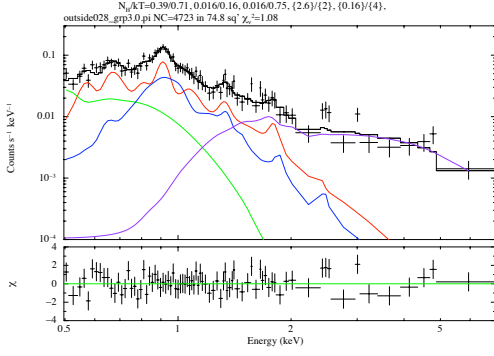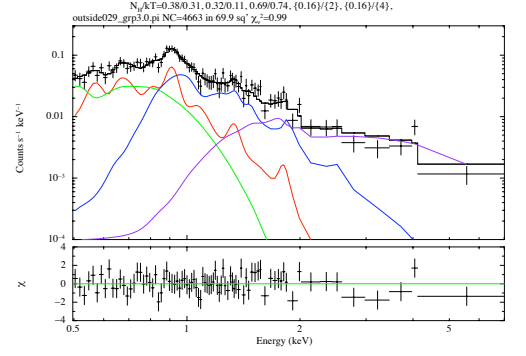

Supplement: Supplementary file 1 [file diffuse_spectra.pdf]
